# Supplementary material for: The Zig-Zag Process and Super-Efficient Sampling for Bayesian Analysis of Big Data
Source: arXiv:1607.03188 ancillary file (2018-04-23)
Supplement: Supplementary file 1 [file supplement.pdf]

Supplement to *The Zig-Zag Process and Super-Efficient Sampling for Bayesian Analysis of Big Data*

Joris Bierkens, Paul Fearnhead, Gareth Roberts

September 25, 2017

# 1 Mathematics of the Zig-Zag process

## 1.1 The Zig-Zag process and its invariant distribution

Here we define the Zig-Zag process via its generator.

For $k \in \{1, \dots, d\}$, let $F_k : \{-1, +1\}^d \to \{-1, +1\}^d$ denote the operation of flipping the $k$-th bit in a binary vector $\theta \in \{-1, +1\}^d$, i.e.

$$(F_k[\theta])_i := \begin{cases} \theta_i & i \neq k \\ -\theta_i & i = k. \end{cases}$$

Let $\lambda \in C(E; \mathbb{R}_+^d)$; we will refer to $\lambda$ as the *switching rate* throughout this paper. Define a densely defined operator $L$ on $C(E)$ by

$$Lf(\xi, \theta) = \sum_{i=1}^d \left\{ \theta_i \partial_i f(\xi, \theta) + \lambda_i(\xi, \theta)(f(\xi, F_i[\theta]) - f(\xi, \theta)) \right\}, \quad (\xi, \theta) \in E, \tag{1}$$

for $f \in C(E)$ such that $f(\cdot, \theta)$ has compact support and is differentiable for all $\theta \in \{-1, +1\}^d$.

The operator $L$, extended to its maximal domain $\mathcal{D}(L)$, is the generator of a piecewise deterministic Markov process satisfying the strong Markov property ([Dav84]).

*Proof of Theorem 2.2 in the paper.* Write $L_i f(\xi, \theta) = \theta_i \partial_i f(\xi, \theta) + \lambda_i(\xi, \theta)(f(\xi, F_i[\theta]) - f(\xi, \theta))$, so that $L = L_1 + \dots + L_d$. Let $f \in \mathcal{D}(L)$. Then for $i = 1, \dots, d$,

$$\begin{aligned}
&\int_E L_i f(\xi, \theta) \, d\mu \\
&= \frac{1}{Z} \sum_{\theta \in \{-1,+1\}^d} \int_{\mathbb{R}^d} \left\{ \theta_i \partial_i f(\xi, \theta) + \lambda_i(\xi, \theta)(f(\xi, F_i[\theta]) - f(\xi, \theta)) \right\} \exp(-\Psi(\xi)) \, d\xi \\
&= \frac{1}{Z} \sum_{\theta \in \{-1,+1\}^d} \int_{\mathbb{R}^d} \left\{ -\theta_i \partial_i \Psi(\xi) + \lambda_i(\xi, F_i[\theta]) - \lambda_i(\xi, \theta) \right\} f(\xi, \theta) \exp(-\Psi(\xi)) \, d\xi \\
&= 0.
\end{aligned}$$

Hence $\int_E Lf \, d\mu = 0$, which by [EK05, Theorem 4.9.17] establishes invariance of $\mu$. □

*Proof of Proposition 2.3 in the paper.* It is straightforward to verify that if $\lambda$ satisfies Equation (4) (in the paper), with $\gamma$ as specified, then it also satisfies (2) (in the paper). Conversely, suppose $\lambda$ satisfies (2) (in the paper) and define

$$\gamma_i(\xi,\theta) := \lambda_i(\xi,\theta) - (\theta_i \partial_i \Psi(\xi))^+, \quad i = 1,\dots,n, (\xi,\theta) \in E.$$

Then a straightforward computation yields $\gamma_i(\xi,\theta) - \gamma_i(\xi, F_i[\theta]) = 0$. Now suppose for some $(\xi,\theta) \in E$, and $i = 1,\dots,n$, $\gamma_i(\xi,\theta) < 0$. First suppose $\theta_i\partial_i\Psi(\xi) \le 0$. Then $\lambda_i(\xi,\theta) = \gamma_i(\xi,\theta) + 0 < 0$ which is in contradiction with the requirement that $\lambda_i(\xi,\theta) \ge 0$. On the other hand, if $\theta_i\partial_i\Psi(\xi) > 0$, then $\lambda_i(\xi, F_i[\theta]) = \gamma_i(\xi, F_i[\theta]) + 0 = \gamma_i(\xi,\theta) < 0$, again a contradiction. It follows that $\gamma_i(\xi,\theta) \ge 0$ for all $i = 1,\dots,n$, $(\xi,\theta) \in E$. □

*Remark* 1.1. The definition of the Zig-Zag process can be extended to have different speed in different directions, i.e. with a generator of the form

$$Lf(\xi,\theta) = \sum_{i=1}^d \left\{\theta_i a_i \partial_i f(\xi,\theta) + \lambda_i(\xi,\theta)(f(\xi,F_i[\theta]) - f(\xi,\theta))\right\}, \quad (\xi,\theta) \in E, \varphi \in \mathcal{D}(L),$$

where $a_i > 0$ for $i = 1,\dots,d$. In this case $\mu$ as in Theorem 2.2 (in the paper) is invariant if and only if

$$\lambda_i(\xi,\theta) - \lambda_i(\xi,F_i[\theta]) = a_i\partial_i\Psi(\xi).$$

Note that after a rescaling the Zig-Zag process with generator (1) is obtained. We will not consider this additional flexibility in this paper to keep the exposition as simple as possible.

## 1.2 Ergodicity

**Lemma 1.2.** *Suppose $\pi^k$ is given as the product of measures, $\pi^k := \pi_1^k \otimes \cdots \otimes \pi_d^k$, with $\pi_i^k$ probability measures on Borel spaces $E_i$ for $k \in \mathbb{N}$ and fixed $d \in \mathbb{N}$, $d \ge 2$. Suppose for every $i = 1,\dots,d$ there exists a measure $\pi_i$ such that $\lim_{k\to\infty} \|\pi_i^k - \pi_i\|_{\mathrm{TV}} = 0$. Then*

$$\lim_{k\to\infty} \|\pi^k - \bigotimes_{i=1}^d \pi_i\|_{\mathrm{TV}} = 0.$$

For $f \in C_b(E)$, with $E$ a topological space, let $\|f\|$ denote the supremum norm of $f$.

*Proof.* It suffices to prove the result for $d = 2$. Write $E = E_1 \times E_2$. For $f \in C_b(E)$, $\|f\| \le 1$, define $h_f^k(x_1) := \int_E f(x_1,y_2)\, d\pi_2^k(y_2)$. Note that for any such $f$ and $k \in \mathbb{N}$, $h_f^k \in C_b(E_1)$ with $\|h_f^k\| \le 1$. Therefore, as $k \to \infty$,

$$\begin{aligned}
&\sup_{\substack{f\in C_b(E)\\ \|f\|\le 1}} |(\pi_1^k \otimes \pi_2^k)(f) - \pi_1(h_f^k)| \\
&= \sup_{\substack{f\in C_b\\ \|f\|\le 1}} \left|\int_{E_1}\int_{E_2} f(y_1,y_2)\ d\pi_1^k(y_1) d\pi_2^k(y_2) - \pi_1(h_f^k)\right| \\
&= \sup_{\substack{f\in C_b(E)\\ \|f\|\le 1}} \left|\int_{E_1} h_f^k\ d\pi_1^k - \pi_1(h_f^k)\right| \le \sup_{\substack{h\in C_b(E)\\ \|h\|\le 1}} \left|\int_{E_1} h\ d\pi_1^k - \pi_1(h)\right| \to 0.
\end{aligned} \tag{2}$$

Also, for any $y_1 \in E_1$, $f(y_1, \cdot) \in C_b(E_2)$ with supremum norm less than or equal to one. Therefore, for all $y_1 \in E_1$, as $k \to \infty$,

$$\begin{aligned}
H^k(y_1) &:= \sup_{\substack{f \in C_b(E) \\ \|f\| \leq 1}} \left| \int_{E_2} f(y_1, y_2)\ d\pi_2^k(y_2) - \int_E f(y_1, y_2)\pi(dy_2) \right| \\
&\leq \sup_{\substack{g \in C_b(E_2) \\ \|g\| \leq 1}} \left| \int_{E_2} g\ d\pi_2^k - \int_{E_2} g\ d\pi_2 \right| \to 0.
\end{aligned}$$

Hence by bounded convergence, as $k \to \infty$,

$$\begin{aligned}
&\sup_{\substack{f \in C_b(E) \\ \|f\| \leq 1}} |\pi_1(h_f^k) - (\pi_1 \otimes \pi_2)(f)| \\
&= \sup_{\substack{f \in C_b(E) \\ \|f\| \leq 1}} \left| \int_{E_1} \left\{ \int_{E_2} f(y_1, y_2)\ d\pi_2^k(y_2) - \int_{E_2} f(y_1, y_2)\ d\pi_2(y_2) \right\} d\pi_1(y_1) \right| \\
&\leq \int_{E_1} \sup_{\substack{f \in C_b(E) \\ \|f\| \leq 1}} \left| \int_{E_2} f(y_1, y_2)\ d\pi_2^k(y_2) - \int_{E_2} f(y_1, y_2)\ d\pi_2(y_2) \right| d\pi_1(y_1) \\
&= \int_{E_1} H^k\ d\pi_1 \to 0.
\end{aligned} \tag{3}$$

Combining (2) and (3) gives, for any $(x_1, x_2) \in E$,

$$\begin{aligned}
\|\pi^k - \pi_1 \otimes \pi_2\|_{\mathrm{TV}} &= \sup_{\substack{f \in C_b(E) \\ \|f\| \leq 1}} |\pi^k(f) - (\pi_1 \otimes \pi_2)(f)| \\
&\leq \sup_{\substack{f \in C_b(E) \\ \|f\| \leq 1}} |(\pi_1^k \otimes \pi_2^k)(f) - \pi_1(h_f^k)| + \sup_{\substack{f \in C_b(E) \\ \|f\| \leq 1}} |\pi_1(h_f^k) - (\pi_1 \otimes \pi_2)(f)| \to 0.
\end{aligned}$$

□

A discrete time Markov chain in $E$ with transition kernel $P$ is called $\varphi$-irreducible if there exists a non-trivial Borel measure $\varphi$ on $E$ such that, whenever $\varphi(A) > 0$ for $A \in \mathcal{B}(E)$ and $x \in E$, there exists a $k \in \mathbb{N}$ such that $P^k(x, A) > 0$.

**Lemma 1.3.** *Suppose the Markov chain on $E$ with transition kernel $P(x, dy)$ is mixing with respect to its unique invariant probability distribution $\pi$. Then the transition kernel $P$ is $\pi$-irreducible.*

*Proof.* Let $A \in \mathcal{E}$ such that $\pi(A) > 0$. Since the Markov chain is mixing, there exists a $k$ such that $|P^k(x, A) - \pi(A)| < \pi(A)/2$, so that $P^k(x, A) > 0$. □

***Proof of Theorem 2.11 of the paper.*** Let $(N_1(t), \ldots, N_d(t))$ denote $d$ independent Poisson processes, each with constant rate $\gamma > 0$ defined on a filtered probability space $(\Omega, \mathcal{F}, (\mathcal{F}_t), \mathbb{Q})$. Given $(\xi, \theta) \in E$, define a stochastic processes $\Theta_i(t; \xi, \theta) := (-1)^{N_i(t)}\theta_i$ for $i = 1, \ldots, d$ and let $\Xi_i(t; \xi, \theta) := x_i + \int_0^t \Theta_i(s; \theta)\ ds$. Then under $\mathbb{Q}$, $(\Xi(\cdot; \xi, \theta), \Theta(\cdot; \xi, \theta))$ corresponds to a Zig-Zag process started in $(\xi, \theta)$ with constant switching rate $\gamma$. Denote the transition kernel for this process by $Q^t((\xi, \theta), \cdot)$.

Write $\lambda(s;\xi,\theta) := \lambda(\Xi(s;\xi,\theta),\Theta(s;\xi,\theta))$. For $(\xi,\theta) \in E$ define a stochastic process $Z(t;\xi,\theta)$ on $(\Omega,\mathcal{F},(\mathcal{F}_t))$ by

$$Z(t;\xi,\theta) = \exp\left(\sum_{i=1}^{d}\int_0^t \log\left(\frac{\lambda_i(s;\xi,\theta)}{\gamma}\right)\, dN_i(s) - \sum_{i=1}^{d}\int_0^t \{\lambda_i(s;\xi,\theta)-\gamma\}\, ds\right),$$

Since $\lambda_i(s;\xi,\theta) > 0$ for all $i = 1,\dots,d$, $s \geq 0$, and $(\xi,\theta) \in E$, it follows that $\lambda_i(\Xi(s;\xi,\theta),\Theta(s;\xi,\theta))$ is bounded away from 0 for all $i = 1,\dots,d$ and $0 \leq s \leq t$. Using this local boundedness property the processes $(Z(\cdot;\xi,\theta))$ are a.s. positive martingales. For fixed $(\xi,\theta)$, the probability measure $\mathbb{P}_{\xi,\theta}$ on $\mathcal{F}_t$, defined by the Radon-Nikodym derivative

$$\left.\frac{d\mathbb{P}_{\xi,\theta}}{d\mathbb{Q}}\right|_{\mathcal{F}_t} = Z(t;\xi,\theta)$$

is such that under $\mathbb{P}_{\xi,\theta}$, the processes $N_i(s)$ have time inhomogeneous rate $\lambda_i(\Xi(s;\xi,\theta),\Theta(s;\xi,\theta))$. Let $P^t((\xi,\theta),\cdot)$ denote the probability distribution of $(\Xi(t),\Theta(t))$ under $\mathbb{P}$, and similarly $Q^t$ for the distribution under $\mathbb{Q}$ for $t \geq 0$. Then

$$P^t((\xi,\theta),A) = \mathbb{E}^{\mathbb{Q}}\left[Z(t;\xi,\theta)\mathbb{1}_A(\Xi(t;\xi,\theta),\Theta(t;\xi,\theta))\right],$$

whence for all $(\xi,\theta)$ and $t \geq 0$, $P^t((\xi,\theta),\cdot)$ and $Q^t((\xi,\theta),\cdot)$ are equivalent.

Now take $\widetilde{\lambda}$ to be equal to the switching rates for a standard normal target distribution with excessive switching rate $\gamma$, i.e.

$$\widetilde{\lambda}_i(\xi,\theta) = (\theta_i x_i)^+ + \gamma,$$

and repeat the above construction to obtain transition probabilities $\widetilde{P}^t((\xi,\theta),\cdot)$. It follows that the transition probabilities $P^t$ and $\widetilde{P}^t$ are equivalent for all $t \geq 0$ and $(\xi,\theta) \in E$. From Proposition 2.9 and Example 2.7 (in the paper) it follows that the time discretization of the Zig-Zag process with transition kernels $(\widetilde{P}^{\delta k})$ is mixing. By Lemma 1.3, it follows that the transition kernels $(\widetilde{P}^{\delta k})$ correspond to a $\varphi$-irreducible process. By the equivalence of the transition kernels $P^t$ and $\widetilde{P}^t$, this property carries over the the Zig-Zag process with switching rates $\lambda$. It follows that there can be at most a single unique invariant distribution for the time discretization of the Zig-Zag process, and this property carries over to the continuous time Zig-Zag process. □

# 2 Effective Sample Size for continuous time trajectories

In order to perform numerical experiments we compute, for an obtained continuous time Zig-Zag trajectory $(\Xi(t),\Theta(t))$, the associated Effective Sample Size (ESS) corresponding to a continuous observable $h : \mathbb{R}^d \to \mathbb{R}$. We say that the Central Limit Theorem (CLT) holds for $(h(\Xi(t)))_{t\geq 0}$ if, as $t \to \infty$, the distribution of

$$\frac{1}{\sqrt{t}}\int_0^t \{h(\Xi(s)) - \pi(h)\}\, ds$$

converges in distribution to a centred normal distribution with variance $\sigma_h^2$, called the *asymptotic variance*. The asymptotic variance can be estimated by dividing an obtained trajectory $(\Xi(t))_{0\leq t\leq\tau}$ into $B$ intervals ("batches") of length $\tau/B$. Under the assumption that the batch are sufficiently large, we have that

$$Y_i := \sqrt{\frac{B}{\tau}}\int_{(i-1)\tau/B}^{i\tau/B} h(\Xi(s))\, ds$$

has approximately a $N\left(\sqrt{\frac{\tau}{B}}\pi(h), \sigma_h^2\right)$ distribution, for $i = 1, \ldots, B$. Making the further approximating assumption that the random variables $(Y_i)$ are independent (which is reasonable if the batches themselves are sufficiently long), we may estimate $\sigma_h^2$ as the sample variance of $(Y_i)_{i=1,\ldots,B}$, i.e. we use the estimator

$$\widehat{\sigma_h^2} = \frac{1}{B-1}\sum_{i=1}^{B}(Y_i - \overline{Y})^2,$$

with $\overline{Y} = \frac{1}{B}\sum_{i=1}^{B} Y_i$. We also estimate the mean and variance of $h$ under $\pi$ by

$$\widehat{\pi(h)} := \frac{1}{\tau}\int_0^\tau h(\Xi(s))\, ds, \quad \widehat{\operatorname{Var}_\pi h} := \frac{1}{\tau}\int_0^\tau h(\Xi(s))^2\, ds - \left(\widehat{\pi(h)}\right)^2,$$

which converge almost surely as $\tau \to \infty$ to the true mean and variance under the condition that the Zig-Zag process is ergodic. The estimate for Effective Sample Size is now given as

$$\widehat{ESS} := \frac{\tau \widehat{\operatorname{Var}_\pi(h)}}{\widehat{\sigma_h^2}}.$$

# 3 Scaling of Stochastic Gradient Langevin Dynamics for large datasets

For notational simplicity we will focus on a 1-dimensional target, though the arguments below apply more generally. The SGLD algorithm consists of stochastic updates of the form

$$\Xi_i := \Xi_{i-1} + \tfrac{1}{2} h_i \widehat{\nabla_\xi \log}\, \pi(\Xi_{i-1}) + \sqrt{h_i} Z_i, \tag{4}$$

where $(h_i)$ is a sequence of positive step sizes, $(Z_i)$ are independent $N(0,1)$ random variables, and where $\widehat{\log \pi}(\xi)$ is an unbiased estimator of $\log \pi(\xi)$ for $\xi \in \mathbb{R}^d$. In practice, $\widehat{\nabla \log \pi}$ will be constructed using randomly sampled batches of fixed size $m \in \{1, \ldots, n\}$,

$$\widehat{\nabla \log \pi}(\xi) := \frac{n}{m}\sum_{i=1}^{m} \nabla_\xi \left(\frac{1}{n}\log \pi_0(\xi) + f(x^{J_i} \mid \xi)\right),$$

where $(J_i)_{i=1}^m$ are drawn uniformly without replacement from $\{1, \ldots, n\}$. Under certain conditions, in particular on the decay of the step sizes to 0 as $i \to \infty$, SGLD provides an asymptotically unbiased approximation of the target distribution $\pi$; see [TTV14] for a detailed analysis. However the Monte Carlo error of the resulting algorithm decays at a slower rate than for standard MCMC algorithms. We implement with a fixed step size (as in [VZT15]) as is done in practice and which makes the comparison with the Zig-Zag algorithms more straightforward.

As in Section 5 (of the paper) it is natural to study the behaviour of SGLD for a scaled variable, $\phi(\xi) := \sqrt{n}(\xi - \widehat{\xi})$, that converges to a fixed distribution as $n \to \infty$. With respect to the reparametrization $\phi$, the updates (4) correspond to

$$\Phi_i := \Phi_{i-1} + \tfrac{1}{2} hn \widehat{\nabla_\phi \log}\, \pi(\Phi_{i-1}) + \sqrt{hn} Z_i,$$

with $\xi(\phi) := \widehat{\xi}_n + n^{-1/2}\phi$. We see that $h$ has to scale as $O(n^{-1})$ in order for the noise to be of $O(1)$ in the $\phi$-coordinate. Therefore we let $h := c_1/n$ for some $c_1 > 0$.

The error of using the SGLD algorithm with a fixed step-size $h_i = h$ is analysed in [VZT15]. To first order the error is governed by the relative sizes of the variance of the estimator of the drift and the variance of the driving noise. Furthermore, it is possible to correct for this error providing the latter variance is greater than the former.

First we calculate the variance of the estimator of the drift. Define $\sigma > 0$ by

$$\mathrm{Var}\left(\nabla_\xi f(x^J \mid \xi)\right) = \sigma^2,$$

where the variance is with respect to the randomness induced by $J$, drawn uniformly among $\{1, \ldots, n\}$. Then by the expression for the variance for sampling without replacement [Ric06, Section 7.3.1], and using $\sqrt{n}\nabla_\phi \log \pi = \nabla_\xi \log \pi$,

$$\mathrm{Var}\left(h\sqrt{n}\widehat{\nabla_\xi \log \pi}\right) = h^2 n^3 \,\mathrm{Var}\left(\frac{1}{m}\sum_{i=1}^{m} \nabla_\xi \left(f(x^{J_i} \mid \xi)\right)\right) = \frac{c_1^2 n \sigma^2}{m}\left(\frac{n-m}{n-1}\right).$$

This is $O(n/m)$. By comparison the variance of the driving noise is $O(1)$. If we want the former to be less than the latter we will need $m$ to be $O(n)$. That is we will need to sub-sample a fixed proportion of the data at each iteration. We therefore choose a sub-sample of size $c_2 n$. Thus the advantage of SGLD over a method that does not use sub-sampling can at best be by a constant factor, and SGLD cannot be super-efficient. The only potential to develop SGLD to be super-efficient would be to substantially reduce the variance of the estimator of the drift, for example by using the control variate idea we use within ZZ-CV; see also [HZ16].

# 4 Details on estimating the mean of a Gaussian

We assume that conditional on a parameter $\xi \in \mathbb{R}^d$, independent observations $(x^j)_{j=1}^n$ have distribution $N(\xi, \sigma^2)$. In the experiment data $(x^j)_{j=1}^n$ is generated from $N(\xi_0, \sigma^2)$. We put a prior distribution $\pi_0 \sim N(0, \rho^2)$ on $\xi$. This leads to a prior distribution $\pi(\xi) \propto \exp(-\Psi(\xi))$ with negative log density

$$\Psi(\xi) = \frac{\|\xi\|^2}{2\rho^2} + \frac{1}{2\sigma^2}\sum_{j=1}^{n} \|\xi - x^j\|^2, \quad \xi \in \mathbb{R}^d.$$

We compute

$$\nabla\Psi(\xi) = \left(\frac{1}{\rho^2} + \frac{n}{\sigma^2}\right)\xi - \frac{1}{\sigma^2}\sum_{j=1}^{n} x^j, \quad \xi \in \mathbb{R}^d$$

and

$$H_\Psi(\xi) = \left(\frac{1}{\rho^2} + \frac{n}{\sigma^2}\right) I, \quad \xi \in \mathbb{R}^d.$$

For any trajectory $\xi(t) = \xi + \theta t$, we have

$$\lambda_i(\xi(t), \theta) = \max\left(0, \theta_i \partial_i \Psi(\xi + \theta t)\right) = \max\left(0, a_i + b_i t\right) =: M_i(t),$$

with

$$a_i = \theta_i \frac{\xi_i}{\rho^2} + \frac{\theta_i}{\sigma^2}\sum_{j=1}^{n}[\xi_i - x_i^j] \quad \text{and} \quad b_i = \frac{1}{\rho^2} + \frac{n}{\sigma^2}, \quad i = 1, \ldots, d.$$

We see that in this case we can construct computational bounds $(M_i(t))$ which are exact, so that all proposed switching times will be accepted. The corresponding algorithm will be simply denoted by ZZ.

Since there is no global bound on the switching rate there is no straightforward way to implement the naive sub-sampling method of Section 4.2 (in the paper). However, because the Hessian of $\Psi$ is constant it is possible to apply the sub-sampling method with control variates of Section 4.3 (in the paper). In fact, because the data has an additive effect on the gradient of $\Psi$, we have for arbitrary $\xi^\star$ that

$$E_i^j(\xi) = \partial_i \Psi(\xi^\star) + \partial_i \Psi^j(\xi) - \partial_i \Psi^j(\xi^\star) = \partial_i \Psi(\xi), \quad \xi \in \mathbb{R}^d,$$

we see that the sub-sampling switching rates are exactly equal to the canonical switching rates, and the two continuous time stochastic processes coincide, once we note that we can pre-compute $\sum_{j=1}^n x^j$ in the expression for $\nabla \Psi(\xi)$.

However the computational bounds of the two algorithms are not equal, and it will be of interest to see how Zig-Zag with control variates behaves if $\xi^\star$ is not chosen to be exactly equal to the mode. The mode of $\pi$ is given by

$$\xi^{\mathrm{MAP}} = \frac{\frac{1}{n}\sum_{j=1}^n x^j}{1 + \frac{\sigma^2}{n\rho^2}},$$

and the one-off cost of computing this quantity is $O(n)$. Alternatively we can choose to use a sub-sampling of $(x^j)$ to obtain a value $\xi^\star$ close to the posterior mode. As we require $\xi^\star$ to be within $O(n^{-1/2})$ of the mode, the size of such a sample should be at least proportional to $n$. To be specific, we will consider the case where $\xi^\star$ is determined randomly by

$$\xi^\star = \frac{\frac{1}{m}\sum_{j=1}^m x^{J_j}}{1 + \frac{\sigma^2}{n\rho^2}},$$

where $m = \lceil cn \rceil$ for some constant $c \in (0, 1]$, and $(J^i)_{i=1}^m$ are drawn randomly without replacement from $\{1, \ldots, m\}$. The corresponding Zig-Zag algorithms are denoted by ZZ-soCV (sub-optimal Control Variates, for $\xi^\star$ an approximation to the mode), and ZZ-CV (for $\xi^\star = \xi^{\mathrm{MAP}}$).

The constants $(C_i)$ determining the computational bounds (as described in Section 4.3 in the paper) are given by $C_i = \frac{1}{\rho^2} + \frac{n}{\sigma^2}$ for $i = 1, \ldots, d$, regardless of the choice of $p \in [1, \infty]$. Choosing $p = \infty$ will give optimal scaling of $a_i$ and $b_i$ with respect to dimension in the computational bound $M_i(t) = \max(0, a_i + b_i t)$.

# 5 Details on logistic regression

Consider a binary data set $y^j \in \{0, 1\}$, $j = 1, \ldots, n$ given $d$-dimensional covariates $x^j \in \mathbb{R}^d$, $j = 1, \ldots, n$ (with $x_1^j = 1$ for all $j$) assumed to come from the logistic regression model,

$$\mathbb{P}(y = 1 \mid x, \xi) = \frac{1}{1 + \exp(-\sum_{i=1}^d \xi_i x_i)},$$

with parameter $\xi \in \mathbb{R}^d$. For any given prior probability distribution $\pi_0$ on the value of $\xi$, we obtain for the posterior density function

$$\pi(\xi) = \pi_0(\xi) \prod_{j=1}^n \frac{\exp\left(y^j \sum_{i=1}^d x_i^j \xi_i\right)}{1 + \exp\left(\sum_{i=1}^d x_i^j \xi_i\right)}, \quad \xi \in \mathbb{R}^d.$$

For simplicity we assume a flat prior on $\xi \in \mathbb{R}^d$, i.e. $\pi_0$ is constant. The corresponding negative log density function is now given by

$$\Psi(\xi) = \sum_{j=1}^{n} \left\{ \log\left(1 + \exp\left(\sum_{i=1}^{d} x_i^j \xi_i\right)\right) - y^j \sum_{i=1}^{d} x_i^j \xi_i \right\}, \quad \xi \in \mathbb{R}^d.$$

For the $k$-th derivative we find

$$\partial_k \Psi(\xi) = \sum_{j=1}^{n} \left\{ \frac{x_k^j \exp\left(\sum_{i=1}^{d} x_i^j \xi_i\right)}{1 + \exp\left(\sum_{i=1}^{d} x_i^j \xi_i\right)} - y^j x_k^j \right\}, \quad \xi \in \mathbb{R}^d.$$

In order to prepare for sub-sampling, we can write $\Psi = \frac{1}{n}\sum_{j=1}^{n} \Psi^j$, with

$$\Psi^j(\xi) = n \log\left(1 + \exp\left(\sum_{i=1}^{d} x_i^j \xi_i\right)\right) - n y^j \sum_{i=1}^{d} x_i^j \xi_i, \quad \xi \in \mathbb{R}^d, \quad j = 1, \ldots, n.$$

We compute for $j = 1, \ldots, n$,

$$\partial_k \Psi^j(\xi) = \frac{n x_k^j \exp\left(\sum_{i=1}^{d} x_i^j \xi_i\right)}{1 + \exp\left(\sum_{i=1}^{d} x_i^j \xi_i\right)} - n y^j x_k^j, \quad \xi \in \mathbb{R}^d, \quad k = 1, \ldots, d, \tag{5}$$

and

$$\partial_k \partial_l \Psi^j(\xi) = \frac{n x_k^j x_l^j \exp\left(\sum_{i=1}^{d} x_i^j \xi_i\right)}{\left(1 + \exp\left(\sum_{i=1}^{d} x_i^j \xi_i\right)\right)^2}, \quad \xi \in \mathbb{R}^d, \quad k, l = 1, \ldots, d.$$

Using the estimate $0 < \exp(a)/(1 + \exp(a)) < 1$, we find that the global bound (equation (12) in the paper) holds with

$$c_i := n \max_{j=1,\ldots,n} |x_i^j|,$$

so that we can use the sub-sampling method with a global bound on the switching rate, discussed in Section 4.2 (in the paper). Furthermore, using the bound $\exp(a)/(1+\exp(a))^2 \leq 1/4$, we have

$$H_\Psi(\xi) \preceq Q := \frac{1}{4} \sum_{j=1}^{n} x^j (x^j)^\top,$$

so that we can use the Zig-Zag algorithm for dominated Hessian (without sub-sampling), discussed in Section 3.3 (in the paper). Finally, using analogous estimates, we find that

$$\partial_k \partial_l \Psi^j(\xi)| \leq n |x_k^j x_l^j|/4, \quad \xi \in \mathbb{R}^d, \quad k, l = 1, \ldots, d,$$

from which it follows that equation (13) (in the paper) is satisfied with

$$C_i := n \max_{j=1,\ldots,n} \frac{1}{4} |x_i^j| \|x^j\|_2, \quad i = 1, \ldots, d, \tag{6}$$

enabling the use of the sub-sampling method with control variates, discussed in Section 4.3 in the paper.

*Remark* 5.1. If $x^j$ are drawn independently from any (sub-)Gaussian distribution, taking the maximum in (6) results in $C_i = O(n \log n)$, using e.g. [Han14, Lemma 5.1]. If on the other hand all $x^j$ are taken (not necessary independently) from a bounded set, then trivially $C_i = O(n)$.

# 6 Details on non-identifiable logistic regression

We have in general in a usual logistic regression problem

$$p(y=1 \mid x,\xi) = \frac{1}{1+\exp\left(-\sum_{i=0}^{d} \xi_i x_i\right)} \quad \text{and} \quad p(y=0 \mid x,\xi) = 1 - p(y=1 \mid x,\xi).$$

However, now assume we have a slightly more complex, non-linear dependence on parameters $\xi = (\xi_1, \xi_2)$, of the following form,

$$p(y=1 \mid x,\xi) = \frac{1}{1+\exp\left(-(\xi_1+\xi_2^2)x\right)}.$$

Taking a Gaussian prior $\mathcal{N}(0, \frac{1}{\rho} I)$, we find

$$\Psi(\xi) = \frac{\rho}{2}\|\xi\|^2 + \sum_{i=1}^{n}\left\{\log\left(1+\exp\left((\xi_1+\xi_2^2)x^i\right)\right) - y^i(\xi_1+\xi_2^2)x^i\right\}.$$

We find

$$\nabla\Psi(\xi) = \rho\xi + \sum_{i=1}^{n}\left\{\frac{1}{h^i(\xi)} - y^i\right\}\begin{pmatrix} x^i \\ 2\xi_2 x^i \end{pmatrix}, \tag{7}$$

where $h^i(\xi) = 1+\exp\left(-(\xi_1+\xi_2^2)x^i\right)$. For the switching rates we find

$$\lambda_1(\xi,\theta) = \left(\theta_1\left[\rho\xi_1 + \sum_{i=1}^{n}\left\{\frac{1}{h^i(\xi)} - y^i\right\}x^i\right]\right)^+,$$

$$\lambda_2(\xi,\theta) = \left(\theta_2\left[\rho\xi_2 + 2\xi_2\sum_{i=1}^{n}\left\{\frac{1}{h^i(\xi)} - y^i\right\}x^i\right]\right)^+.$$

It may be verified that $h^i(\xi) \in (1,\infty)$ for all $i,\xi$ and therefore $\left|\frac{1}{h^i(\xi)} - y^i\right| \le 1$ for all $i,\xi$. Thus we can bound the switching rates along a trajectory $\xi+\theta t$ by

$$\lambda_1(\xi+\theta t,\theta) = \left(\theta_1\left[\rho(\xi_1+\theta_1 t) + \sum_{i=1}^{n}\frac{1-y^i h^i(\xi+\theta t)}{h^i(\xi+\theta t)}x^i\right]\right)^+ \le \left(\theta_1\rho\xi_1 + \sum_{i=1}^{n}|x^i| + \rho t\right)^+,$$

$$\begin{aligned}\lambda_2(\xi+\theta t,\theta) &= \left(\theta_2\left[\rho(\xi_2+\theta_2 t) + 2(\xi_2+\theta_2 t)\sum_{i=1}^{n}\frac{1-y^i h^i(\xi+\theta t)}{h^i(\xi+\theta t)}x^i\right]\right)^+ \\ &\le \left(\theta_2\rho\xi_2 + 2|\xi_2|\sum_{i=1}^{n}|x^i| + \left(\rho + 2\sum_{i=1}^{n}|x^i|\right)t\right)^+.\end{aligned}$$

It is straightforward to numerically invert expressions of the form $(a_0 + a_1 t + \cdots + a_p t^p)^+ = y$, where $a_0 \in \mathbb{R}$ and $a_i \ge 0$, $i = 1,\ldots,p$, $p \in \mathbb{N}$, enabling us to use the CDF inversion technique with the above computational bounds, as well as the bounds obtained in the following section.

## 6.1 Control variates

The potential function for the $j$-th observation $(x^j, y^j)$ is given by

$$\Psi^j(\xi) = \frac{\rho}{2}\|\xi\|^2 + n\left\{\log\left(1+\exp\left((\xi_1+\xi_2^2)x^j\right)\right) - y^j(\xi_1+\xi_2^2)x^j\right\}$$

which has gradient

$$\nabla\Psi^j(\xi) = \rho\xi + n\left\{\frac{1}{h^j(\xi)} - y^j\right\}\begin{pmatrix} x^j \\ 2\xi_2 x^j \end{pmatrix}$$

and Hessian

$$H_{\Psi^j}(\xi) = \rho I + n\begin{pmatrix} \left|\frac{x^j}{h^j(\xi)}\right|^2 \exp(-g(\xi)x^j) & 2\xi_2\left|\frac{x^j}{h^j(\xi)}\right|^2 \exp(-g(\xi)x^j) \\ 2\xi_2\left|\frac{x^j}{h^j(\xi)}\right|^2 \exp(-g(\xi)x^j) & 2\left(\frac{1}{h^j(\xi)} - y^j\right)x^j + 4\left|\frac{\xi_2 x^j}{h^j(\xi)}\right|^2 \exp(-g(\xi)x^j) \end{pmatrix},$$

with $g(\xi) = \xi_1 + \xi_2^2$. It is easily verified that $\frac{a}{(1+a)^2}$ attains it maximum in $a = 1$, and thus $\frac{1}{(h^j(\xi))^2}\exp(-g(\xi)) \leq \frac{1}{4}$. We have

$$\left|\partial_{\xi_k}\frac{1}{h^j(\xi)}\right| = \frac{\exp(-g(\xi)x^j)|\partial_{\xi_k}g(\xi)x^j|}{(1+\exp(-g(\xi)x^j))^2}.$$

Since $\frac{a}{(1+a)^2} \leq \frac{1}{4}$ for $a > 0$, it follows that

$$\left|\partial_{\xi_1}\frac{1}{h^j(\xi)}\right| \leq \frac{|x^j|}{4} \quad \text{and} \quad \left|\partial_{\xi_2}\frac{1}{h^j(\xi)}\right| \leq \frac{|x^j||\xi_2|}{2}.$$

For $\eta \in \mathbb{R}^2$ on the line segment between $\xi + \theta t$ and $\xi^\star$, we have

$$|\eta_2| \leq \max(|\xi_2 + \theta_2 t|, |\xi_2^\star|) \leq \max(|\xi_2|, |\xi_2^\star|) + t.$$

It follows that on this line segment,

$$\left|\partial_{\xi_1}\frac{1}{h^j}\right|(\cdot) \leq \frac{|x^j|}{4} \quad \text{and} \quad \left|\partial_{\xi_2}\frac{1}{h^j}\right|(\cdot) \leq \frac{|x^j|(\max(|\xi_2|, |\xi_2^\star|) + t)}{2}.$$

Thus

$$\begin{aligned}
&\lambda_1^j(\xi + \theta t, \theta) = \left[\theta_1\left\{\partial_{\xi_1}\Psi^j(\xi + \theta t) - \partial_{\xi_1}\Psi^j(\xi^\star)\right\}\right]^+ \\
&= \left[\theta_1\left\{\rho(\xi_1 + \theta_1 t - \xi_1^\star) + nx^j\left(\frac{1}{h^j(\xi + \theta t)} - \frac{1}{h^j(\xi^\star)}\right)\right\}\right]^+ \\
&\leq \left[\theta_1\rho(\xi_1 + \theta_1 t - \xi_1^\star) + n|x^j|^2\left(\frac{|\xi_1 + \theta_1 t - \xi_1^\star|}{4} + \frac{(\max(|\xi_2|, |\xi_2^\star|) + t)|\xi_2 + \theta_2 t - \xi_2^\star|}{2}\right)\right]^+ \\
&\leq \left[a_{1,1}^j + a_{1,2}^j t + a_{1,3}^j t^2\right]^+ =: m_1^j(t),
\end{aligned}$$

with

$$\begin{aligned}
a_{1,1}^j &:= \theta_1\rho(\xi_1 - \xi_1^\star) + n|x^j|^2\left(\frac{|\xi_1 - \xi_1^\star| + 2\max(|\xi_2|, |\xi_2^\star|)|\xi_2 - \xi_2^\star|}{4}\right), \\
a_{1,2}^j &:= \rho + n|x^j|^2\left(\frac{1 + 2(|\xi_2 - \xi_2^\star| + \max(|\xi_2|, |\xi_2^\star|))}{4}\right), \\
a_{1,3}^j &:= \frac{n|x^j|^2}{2}.
\end{aligned}$$

Using that $|ab - cd| \leq |a|\,|b-d| + |a-c|\,|d|$ (with $a = \frac{1}{h^j(\xi+\theta t)} - y^j$, $b = \xi_2 + \theta_2 t$, $c = \frac{1}{h^j(\xi^\star)} - y^j$ and $d = \xi_2^\star$), and $|\frac{1}{h^j(\cdot)} - y^j| \leq 1$,

$$\begin{aligned}
&\lambda_2^j(\xi+\theta t, \theta) = \left[\theta_2 \left\{\partial_{\xi_2}\Psi^j(\xi+\theta t) - \partial_{\xi_2}\Psi^j(\xi^\star)\right\}\right]^+ \\
&= \left[\theta_2 \left\{\rho(\xi_2 + \theta_2 t - \xi_2^\star) + 2nx^j \left(\left(\frac{1}{h^j(\xi+\theta t)} - y^j\right)(\xi_2 + \theta_2 t) - \left(\frac{1}{h^j(\xi^\star)} - y^j\right)\xi_2^\star\right)\right\}\right]^+ \\
&\leq \left[\theta_2\rho(\xi_2 - \xi_2^\star) + \rho t + 2n|x^j| \left(|\xi_2 + \theta_2 t - \xi_2^\star| + \left|\frac{1}{h^j(\xi+\theta t)} - \frac{1}{h^j(\xi^\star)}\right| |\xi_2^\star|\right)\right]^+ \\
&\leq \Bigg[\theta_2\rho(\xi_2 - \xi_2^\star) + \rho t \\
&\quad + 2n|x^j| \left(|\xi_2 - \xi_2^\star| + t + |\xi_2^\star|\,|x^j| \left(\frac{|\xi_1 + \theta_1 t - \xi_1^\star|}{4} + \frac{(\max(|\xi_2|, |\xi_2^\star|) + t)|\xi_2 + \theta_2 t - \xi_2^\star|}{2}\right)\right)\Bigg]^+ \\
&\leq \left[a_{2,1}^j + a_{2,2}^j t + a_{2,3}^j t^2\right]^+ =: m_2^j(t),
\end{aligned}$$

with

$$\begin{aligned}
a_{2,1}^j &:= \theta_2\rho(\xi_2 - \xi_2^\star) + 2n|x^j|\,|\xi_2 - \xi_2^\star| + \frac{n|\xi_2^\star|\,|x^j|^2}{2}\left(|\xi_1 - \xi_1^\star| + 2\max(|\xi_2|, |\xi_2^\star|)|\xi_2 - \xi_2^\star|\right), \\
a_{2,2}^j &:= \rho + 2n|x^j| + n|x^j|^2|\xi_2^\star| \left(\tfrac{1}{2} + |\xi_2 - \xi_2^\star| + \max(|\xi_2|, |\xi_2^\star|)\right), \\
a_{2,3}^j &:= n|x^j|^2|\xi_2^\star|.
\end{aligned}$$

Now upper bounds $m_1(t)$, $m_2(t)$ which are uniform in $j$ can be obtained by maximizing the obtained coefficients with respect to $j$, which in turn depends only on the maximal value of $|x^j|$.

# References


[Dav84] M H A Davis. Piecewise-Deterministic Markov Processes: A General Class of Non-Diffusion Stochastic Models. *Journal of the Royal Statistical Society. Series B (Methodological)*, 46(3):353–388, 1984.

[EK05] Stewart N. Ethier and Thomas G. Kurtz. *Markov Processes: Characterization and Convergence (Wiley Series in Probability and Statistics)*. Wiley-Interscience, 2005.

[Han14] Ramon Van Handel. Probability in High Dimension. *http://www.princeton.edu/ rvan/ORF570.pdf*, 2014.

[HZ16] Jonathan H. Huggins and James Zou. Quantifying the accuracy of approximate diffusions and Markov chains. *arXiv:1605.06420*, may 2016.

[Ric06] John Rice. *Mathematical statistics and data analysis*. Nelson Education, 2006.

[TTV14] Y W Teh, A H Thiery, and Sebastian Vollmer. Consistency and fluctuations for stochastic gradient Langevin dynamics. *arXiv:1409.0578*, 2014.

[VZT15] Sebastian J Vollmer, Konstantinos C Zygalakis, and Yee Whye Teh. Exploration of the (Non-)asymptotic Bias and Variance of Stochastic Gradient Langevin Dynamics. *arXiv preprint arXiv: 1501.00438*, 2015.
